# Supplementary material for: Decorrelating ReSTIR Samplers via MCMC Mutations
Source: arXiv:2211.00166 source file (2022-10-31)
Supplement: Supplementary file 1 [file Appendix1-v1.tex]

\section{Unbiased Contribution Weights and Elimination of Startup Bias}
\label{app:StartupBiasElimination}

\eqref{ModifiedContributionWeight} provides an update rule for the contribution weight $W(x_i)$ of a mutated sample $x_i$ from the Markov chain $x_0, ..., x_i, ...$, generated using the Metropolis Hasting algorithm with the target function $\phat$. Here we prove that this rule yields an unbiased contribution weight for any mutated sample $x_i$, \ie,
\begin{equation}
    \label{eq:UnbiasedContributionWeight}
    \mathbb{E}[f(x_i) W(x_i)] = \int_{\Omega} f(x)\ \diff x.
\end{equation}
We assume that the sample $x_0$ used to initialize the chain has the same support $\Omega$ as that of the target function $\phat$. For us, this is guaranteed by the chained application of RIS with a valid shift mapping in \algref{TemporalReuse}. Any $x_0$ chosen by RIS is not distributed exactly in proportion to $\phat$ (which only happens in the limit of infinite samples)---however, its contribution weight $W(x_0)$ is unbiased \citep[Section 4]{Lin:2022:GRIS} and hence satisfies \eqref{UnbiasedContributionWeight}. Furthermore, as we show next, access to $W(x_0)$ is sufficient to eliminate any startup bias with MH.

Our proof follows the general outline of \citet[Appendix 11.A]{Veach:1998:Robust} for unbiased initialization of Metropolis Light Transport. For \eqref{UnbiasedContributionWeight} to hold, we need to show that the following \emph{weighted equilibrium condition} is satisfied at every MH iteration:
\begin{equation}
    \label{eq:WeightedEquilibriumCondition}
    \int_{\mathbb{R}} w\ p_i(w, x)\ \diff w = \frac{\phat(x)}{\phat(x_0)},
\end{equation}
where $p_i$ is the joint density of the $i$-th sample in the chain and its associated contribution weight $W(x_i) = W(x_0) \frac{\phat(x_0)}{\phat(x_i)}$ from \eqref{ModifiedContributionWeight}. This condition is sufficient for \eqref{UnbiasedContributionWeight} to hold, since
\begin{align}
    \label{eq:UnbiasedContributionWeightProof}
    \mathbb{E}[f(x_i) W(x_i)] &= \int_{\Omega} \int_{\mathbb{R}} w\ \frac{\phat(x_0)}{\phat(x)} f(x)\ p_i(w, x)\ \diff w\ \diff x\\
    &= \int_{\Omega} \left(\int_{\mathbb{R}} w\ p_i(w, x)\ \diff w\right) \frac{\phat(x_0)}{\phat(x)} f(x)\ \diff x\\
    &= \int_{\Omega} f(x)\ \diff x.
\end{align}
\paragraph{Proof} We use induction to prove the weighted equilibrium condition for each MH iteration. For $i = 0$, we know from the definition of an unbiased contribution weight that its expected value equals the reciprocal target distribution \citep[Section 4]{Bitterli:2020:ReSTIR}, \ie,
\begin{equation}
    \label{eq:UnbiasedContributionWeightDefinition}
    \int_{\mathbb{R}} w\ p_0(w \mid x)\ \diff w = \frac{1}{p(x)}.
\end{equation}
Multiplying both sides by $p(x)$ then yields $\int_{\mathbb{R}} w\ p_0(w, x)\ \diff w = 1$, which proves the base case since $\phat(x)/\phat(x_0) = 1$ for $i = 0$.

For $i > 0$, we assume $\int_{\mathbb{R}} w\ p_{i-1}(w, x)\ \diff w = \phat(x)/\phat(x_0)$, and invoke a relationship between the probability densities of samples generated by MH at iterations $i$ and $i-1$ \citep[Page 336]{Veach:1998:Robust}:
\begin{multline}
    \label{eq:PDFRelationMH}
    p_i(x) = p_{i-1}(x)\ +\ \int_{\Omega} \left\{\phat_{i-1}(x) T(x \rightarrow x') a(x \rightarrow x') \right. -\\
    \left.
    \phat_{i-1}(x') T(x' \rightarrow x) a(x' \rightarrow x_i)\right\}\ \diff x'.
\end{multline}
Intuitively, this relation says that to maintain equilibrium at the stationary distribution, $p_i(x)$ should equal $p_{i-1}(x)$ while the terms inside the integral should cancel exactly due to the detailed balance condition (\eqref{DetailedBalance}). We first generalize \eqref{PDFRelationMH} slightly by replacing $p_i(x)$ by $p_i(x, w)$, which is valid since mutations have no affect on the contribution weight of the initial sample in the chain. This yields:
\begin{multline}
    \label{eq:JointPDFRelationMH}
    p_i(x, w) = p_{i-1}(x, w)\ +\ \int_{\Omega} \left\{\phat_{i-1}(x, w) T(x \rightarrow x') a(x \rightarrow x') \right. -\\
    \left.
    \phat_{i-1}(x', w) T(x' \rightarrow x) a(x' \rightarrow x_i)\right\}\ \diff x'.
\end{multline}
We now multiply both sides by $w$ and integrate over $\mathbb{R}$ to obtain:
\begin{multline}
    \label{eq:JointPDFRelationIntegratedMH1}
    \int_{\mathbb{R}} w\ p_i(x, w)\ \diff w = \int_{\mathbb{R}} w\ p_{i-1}(x, w)\ \diff w\ +\\
    \int_{\Omega} \left\{\left(\int_{\mathbb{R}} w\ \phat_{i-1}(x, w)\ \diff w\right) T(x \rightarrow x') a(x \rightarrow x') \right. -\\
    \left.
    \left(\int_{\mathbb{R}} w\ \phat_{i-1}(x', w)\ \diff w\right) T(x' \rightarrow x) a(x' \rightarrow x_i)\right\}\ \diff x'.
\end{multline}
Finally, we substitute in the inductive assumption to get:
\begin{multline}
    \label{eq:JointPDFRelationIntegratedMH2}
    \int_{\mathbb{R}} w\ p_i(x, w)\ \diff w = \frac{\phat(x)}{\phat(x_0)}\ +\
    \int_{\Omega} \left\{\frac{\phat(x)}{\phat(x_0)} T(x \rightarrow x') a(x \rightarrow x') \right. -\\
    \left.
    \frac{\phat(x')}{\phat(x_0)} T(x' \rightarrow x) a(x' \rightarrow x_i)\right\}\ \diff x',
\end{multline}
and complete the proof by applying the detailed balance condition:
\begin{equation}
    \label{eq:JointPDFRelationIntegratedMH3}
    \int_{\mathbb{R}} w\ p_i(x, w)\ \diff w = \frac{\phat(x)}{\phat(x_0)}\ +\ 0.
\end{equation}
